# Supplementary material for: Diffusion-DRF: Free, Rich, and Differentiable Reward for Video Diffusion Fine-Tuning
Source: arXiv:2601.04153 source file (2026-11-03)
Supplement: Supplementary file 1 [file ablation.tex]

\begin{table*}[t]
    % \vspace{\pagetopmargin}
    \vspace{-2mm}
    \centering
    \setlength{\tabcolsep}{5.8pt}
    \scriptsize
    \caption{
        \textbf{Ablation studies on question sets and backprop-steps.}
        We report quantitative results using automatic metrics from VBench-2.0 and VBench~\cite{VBench} based on the prompt set from VBench-2.0.
        Besides the summary metrics, we also report scores of sub-dimensions from VBench that reflect visual quality. 
        All models are trained with $2,000$ steps to ensure a fair comparison. 
        % We also
        % \emph{Human Identity} and \emph{Human Anotomy}
        % which highly related to text-video alignment and physical fidelity. 
         %We achieves similar motion smoothness compared to Vanilla DPO, while consistently outperforms it in visual quality, dynamic degree, and text alignment.
    }
    \vspace{-2mm}
    \begin{tabular}{l|ccccc|ccc}
        \toprule
        \multirow{2}{*}{\textbf{Method}}  & \multicolumn{5}{c}{\textit{VBench-2.0}}& \multicolumn{3}{|c}{\textit{VBench}} \\
        \cmidrule{2-9}
        & \multirow{2}{*}{Creativity} & 
         {Common} & \multirow{2}{*}{Controllability} & Human  & \multirow{2}{*}{Physics} & {Imaging}  & Aesthetic  & Motion \\
         & &Sense & & Fidelity& & Quality & Quality & Smoothness \\
        % & Create & Imaging & Subject & Background & Motion & Dynamic  \\
        % & Quality & Quality & Consistency & Consistency & Smoothness & Degree \\
        \midrule
        % \multicolumn{12}{c}{\textit{Baselines}} \\
        % \midrule
        Baseline & {53.79} & {55.52} & {26.59}& {\bf 80.65} & {48.40} & \underline{60.87} & 45.38 & 97.81\\
        TA & 49.41 & 53.80 & 27.03& 74.88&55.64& 60.35 & 48.55 &   \underline{98.08} \\
        % SFT & 56.16 & 55.54 & 87.94 & 92.42 & 94.44 & \textbf{84.93}  \\
       
        TA + Phy & 50.56 & {\bf 60.12} & 25.72 & 75.57 & \underline{55.78} & 57.15 & 46.05 & 97.75 \\
         TA + VQ & \underline{52.34} & 55.81 & \underline{27.80} & 79.02 & 54.65  & {\bf 61.67} & {\bf 50.98} & 98.00 \\
         %TA +  Phy & { 54.58} & {56.96} & { 27.98} & 80.51 & { 56.85} &56.13 \\
         TA + VQ + Phy & {\bf 54.58} & \underline{56.96} & {\bf 27.98} & \underline{80.51} & {\bf 56.85} & 60.64 &  \underline{50.45} & {\bf 98.10} \\
        \midrule
        $K=2$ & 52.45&57.24&27.45&78.50&56.18& 59.14 &48.33 & 97.58\\
        $K=1$ & 52.95&52.93&25.45&79.49&54.99 &  59.36& 49.70 & 98.10\\

        \bottomrule
    \end{tabular}
    \label{tab:quant-ablation}
    \vspace{-2mm}
    % \vspace{\tablemargin}
\end{table*}
