# Supplementary material for: Diffusion-DRF: Free, Rich, and Differentiable Reward for Video Diffusion Fine-Tuning
Source: arXiv:2601.04153 source file (2026-11-03)
Supplement: Supplementary file 2 [file algorithm.tex]

\begin{algorithm}
\caption{Pseudo-codes of Res18-Gate-ReLU}
\begin{algorithmic}
\label{res18relu}
\STATE \textcolor{blue}{def} Block(x, in\_planes, planes)
    %\STATE \quad \textcolor{g}{$\backslash\backslash$ conv1 = nn.Conv2d( in\_planes, planes, 3, 1, 1 )}
    \STATE \quad out = Conv2d(x, in\_planes, planes, 3, 1, 1) 
    %\textcolor{g}{$\backslash\backslash$ Conv2d with kernel\_size=3, stride=1}
    \STATE \quad out = BatchNorm2d(x)
    \STATE \quad out = ReLU(out) * out
    \STATE \quad out = Conv2d(out, planes, planes, 3, 1, 1) 
    \STATE \quad out = BatchNorm2d(out)
    \STATE \quad out += self.shortcut(x)
    \STATE \quad out = ReLU(out)
    \STATE \quad \textcolor{blue}{return} out
\end{algorithmic}
\end{algorithm}
