# Supplementary material for: Diffusion-DRF: Free, Rich, and Differentiable Reward for Video Diffusion Fine-Tuning
Source: arXiv:2601.04153 source file (2026-11-03)
Supplement: Supplementary file 3 [file fig_training_dyn.tex]

\begin{figure*}[t]
% \vspace{\pagetopmargin}
\vspace{-2mm}
\centering
\includegraphics[width=0.3 \linewidth]{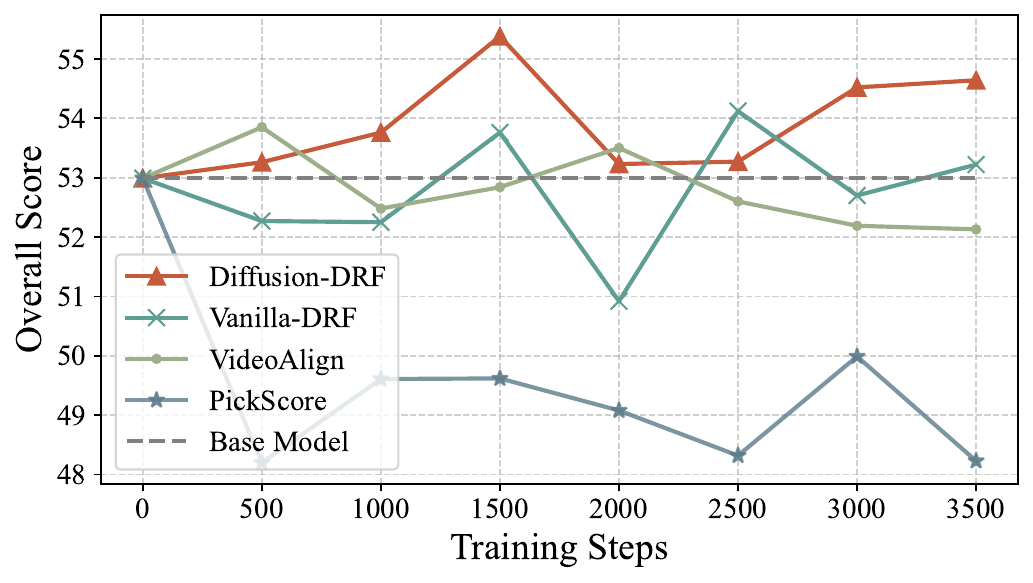}
\includegraphics[width=0.3 \linewidth]{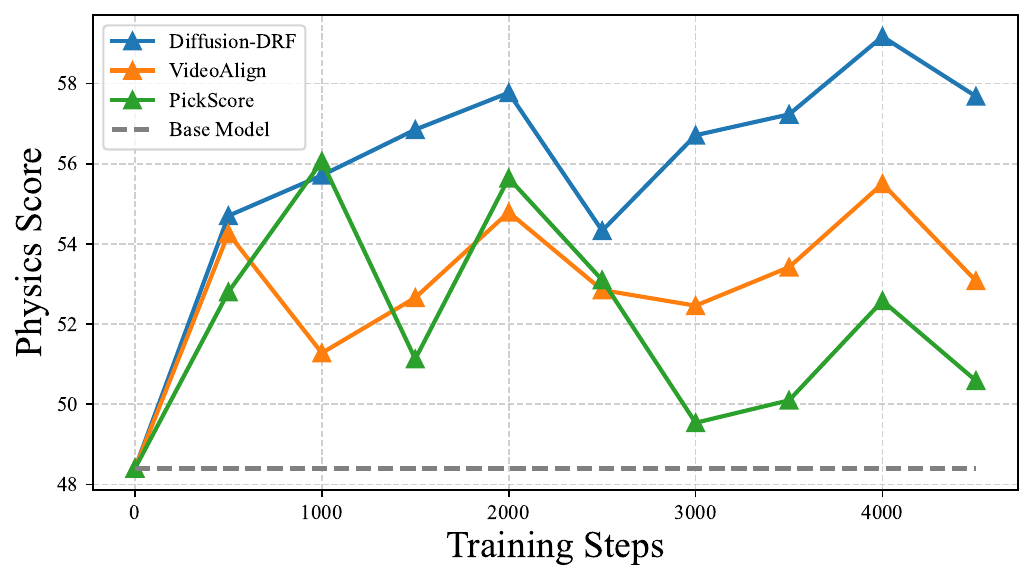}
\includegraphics[width=0.3 \linewidth]{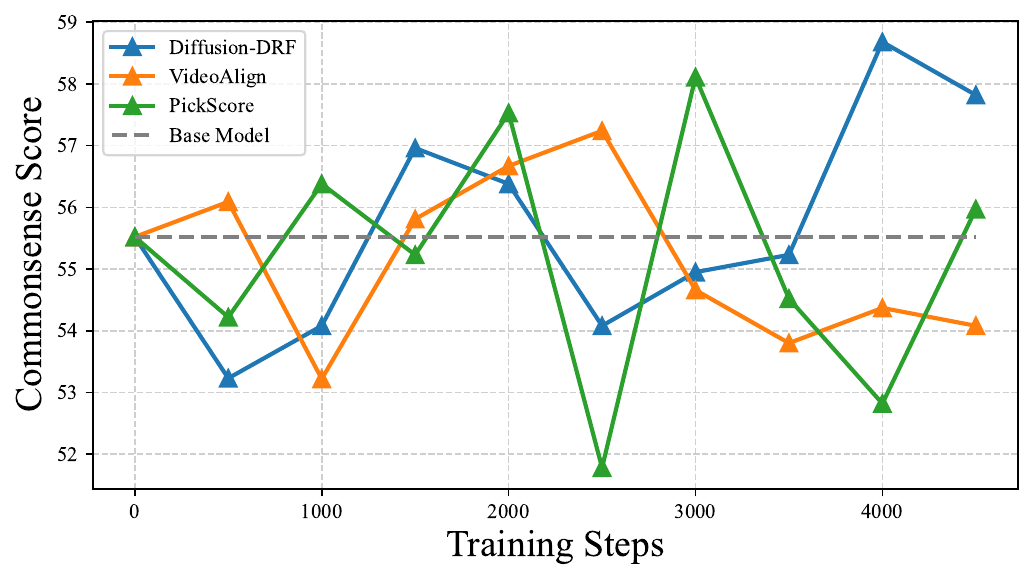}
\includegraphics[width=0.3 \linewidth]{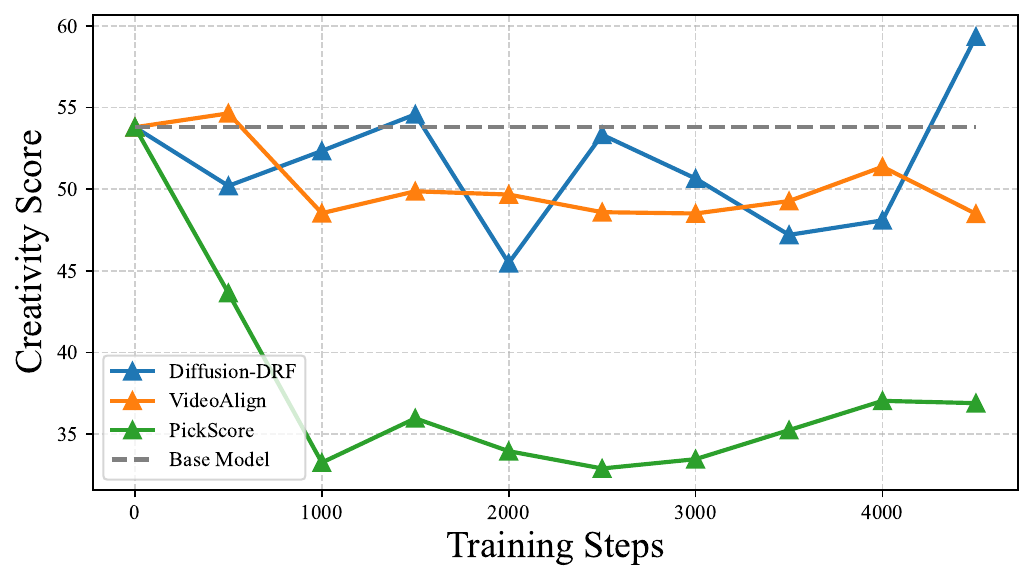}
\includegraphics[width=0.3 \linewidth]{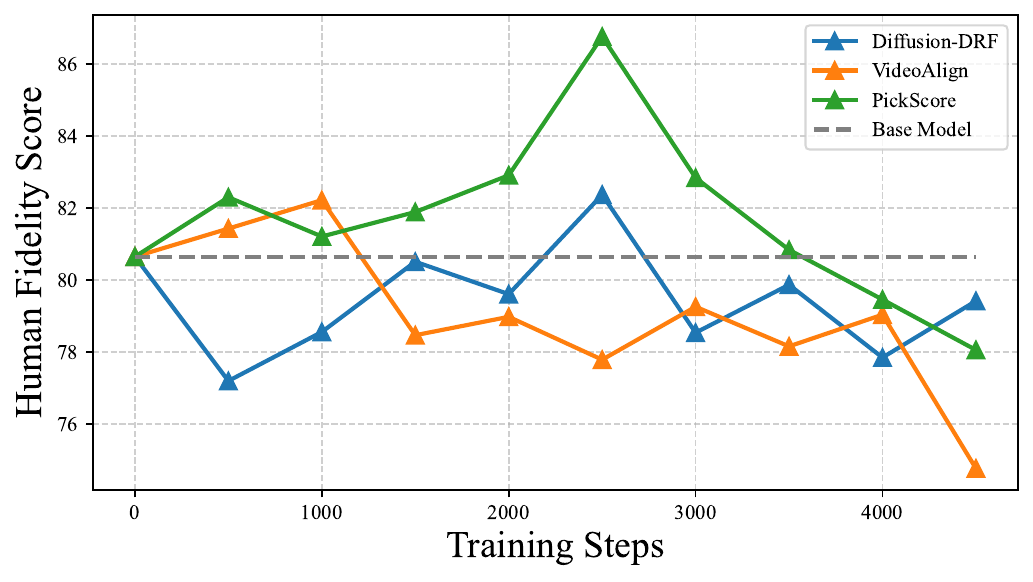}

\caption{
\textbf{Training dynamics} of models trained with different reward models. 
We plot remaining scores using VBench-2.0 metrics. 
Diffusion-DRF shows a more robust training dynamic compared to others.
}
\label{fig:additional_learning_dyn}
% \vspace{2mm}
% \vspace{-10pt}
\end{figure*}
